# Supplementary material for: Photon-starved imaging through turbulence at the diffraction limit
Source: arXiv:2510.22806 source file (2026-10-28)
Supplement: Supplementary file 1 [file Supplementary.pdf]

# Supplementary Information

## Contents

- Section I: Experimental setup and implementation
- Section II: Poisson blind deconvolution algorithm
- Section III: Optical correction for photon-limited imaging
- Section IV: Loss landscape

## I. EXPERIMENTAL SETUP AND IMPLEMENTATION

### A. Optical setup

Figure S1 illustrates the 4f relay optical setup for Turbulence-Aware Poisson blind deconvolution (TAP-BD). The system uses an incoherent LED (M530L4, Thorlabs, CW: 530 nm, FWHM: 35 nm), which passes through a neutral density (ND) filter to simulate low-photon conditions. A narrow bandpass filter (NBP; FLH5532-4, Thorlabs, CW: 532 nm, FWHM: 4 nm) further isolates the desired spectral component. A polarizer ensures that only horizontally polarized light enters the system, aligning with working polarization of the spatial light modulator (SLM).

The light is then focused by lenses L0 and L1 to illuminate the target, with the LED image projected onto the target surface, ensuring the light remains incoherent. The relay system, consisting of lenses L2 and L3, forms an intermediate image after L3. At this stage, Iris1 is introduced for spatial filtering, allowing selective imaging of specific target regions.

Lens L4 performs a Fourier transform of the target image, directing it onto the SLM (E19x12-400-800-HDM8, Meadowlark Optics;  $1920 \times 1200$  pixels, 8  $\mu\text{m}$  pixel pitch). The SLM applies phase modulation composed of three components: a grating phase, turbulence phase, and multiple phase diversity patterns, as described in subsection IB.

The modulated light is then focused by L5, and Iris2 removes unmodulated zero-order diffraction components. The first-order diffraction patterns (with an efficiency of approximately 0.7–0.8) are captured by the EM-CCD (PiMax4: 512EM, Princeton Instruments;  $512 \times 512$  pixels, 24  $\mu\text{m}$  pixel pitch). The magnification is determined by the focal length ratio of L5 to L2. In the configurations used, L5 has a focal length of 20 cm (for Fig. 3 in the main text) or 30 cm (for Fig. 4), while L2 has a focal length of 15 cm, resulting in magnifications of  $1.3 \times$  or  $2.0 \times$ , respectively. All imaging was performed in a darkroom to minimize background light.

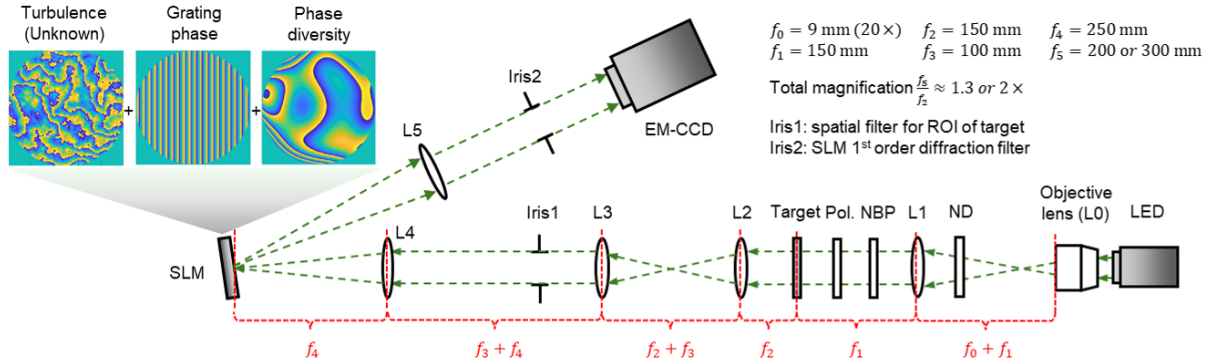

FIG. S1. 4f relay setup with LED illumination and spectral/polarization filtering. incoherent target image is relayed via L2–L5 onto an EM-CCD. A composite phase at the SLM—combining grating, turbulence, and diversity—modulates efield at the Fourier plane. Iris1 selects the region of interest, while Iris2 isolates the 1st-order diffraction.

### B. SLM phase patterns generation

The  $i$ -th SLM phase,  $\Phi_{\text{SLM},i}$  (for  $i = 1, \dots, M$ ), consists of three components:

$$\Phi_{\text{SLM},i} = \Phi_{\text{Grating}} + \Gamma_i + \Phi_{\text{Turbulence}}, \quad (\text{S1})$$

where each component is defined as follows:

1. Grating phase ( $\Phi_{\text{Grating}}$ ): The grating phase  $\Phi_{\text{Grating}}$  spatially separates the 1st-order diffraction patterns from the 0th-order. The blazed grating period  $\Lambda$  is given by:

$$\Lambda = \frac{\lambda \cdot f_5}{d_{\text{shift}} \cdot p_{\text{slm}}}, \quad (\text{S2})$$

where  $\lambda$  is the wavelength,  $f_5$  is the focal length of the imaging lens L5,  $d_{\text{shift}}$  is the lateral shift required to isolate the 1st-order from the 0th-order signal, and  $p_{\text{slm}}$  is SLM pixel size. For our setup,  $\Lambda$  was approximately 3 SLM pixels, corresponding to a lateral shift of about 6 mm when  $f_5 = 30$  cm.

2. Phase diversity ( $\Gamma_i$ ): Phase diversity pattern  $\Gamma_i$  is introduced using the first 15 Zernike polynomials:

$$\Gamma_i = \sum_{n=1}^{15} w_{n,i} Z_n, \quad (\text{S3})$$

where  $\{Z_n\}$  are the Zernike polynomials, and  $\{w_{n,i}\}$  are  $i$ -th Gaussian-distributed random weights with zero mean and variance 20. A total of  $M$  such phase diversity patterns are generated, scaled to the aperture size  $D$ , and zero padded to match the SLM array size.

3. Turbulence Phase ( $\Phi_{\text{Turbulence}}$ ): The turbulence phase  $\Phi_{\text{Turbulence}}$  is the retrieval target. The method for generating  $\Phi_{\text{Turbulence}}$  is detailed in the Appendix or the main text. We refer to  $\Phi_{\text{Turbulence}}$  as  $\Phi$  in subsequent discussions.

To ensure that only the signal inside the aperture contributes to the 1st-order diffraction, the phase outside the aperture with diameter  $D$  is set to zero. This design effectively makes the SLM function as an aperture, preventing unmodulated components from affecting the measurement.

### C. Sample preparation

Three type of samples are used in this work: (1) Negative 1951 USAF target (Thorlab; R3L3S1N), (2) Laser-printed transparent film featuring the Purdue logo, printed at 1200 dpi resolution ( $\sim 0.0212$  mm dot spacing), (3) Beam projector coupled with a  $20 \times$  objective lens to display the Cameraman image. Sample (1) and (2) are located at target location in Fig S1, while sample (3) is placed at L3 in the same figure.

## II. POISSON BLIND DECONVOLUTION ALGORITHM

The TAP-BD framework is designed to jointly reconstruct the target  $O$ , the set of PSFs  $\{h_i\}$ , and the turbulence phase  $\Phi$ , ensuring robust image recovery under challenging low-photon conditions. To achieve this, PBD employs a three-step approach:

1. Poisson denoising: A plug-and-play (PnP) Poisson denoiser is applied to preprocess noisy measurement, mitigating the effects of Poisson shot noise.
2. blind deconvolution (BD): The target  $O$  and the set of PSFs  $\{h_i\}$  are iteratively estimated by enforcing a global consistency constraint on  $O$  across the multiple denoised measurements. BD module is introduced to model the image formation physics, specifically the convolutional relationship between the object and the PSF.
3. turbulence phase retrieval (PR): The turbulence phase  $\Phi$  is refined using the reconstructed PSFs  $\{h_i\}$  from the BD stage and phase diversity patterns  $\Gamma_i$ . This step accounts for wave propagation physics in the PSF. The reconstructed  $\Phi$  is then reintroduced into BD as the updated PSFs model, iteratively refining both the target  $O$  and turbulence phase  $\Phi$ .

Steps (2) and (3) are integrated into each iteration, ensuring a joint optimization process that continuously updates both the object reconstruction and turbulence estimation. The overall workflow is illustrated in Figure S2.

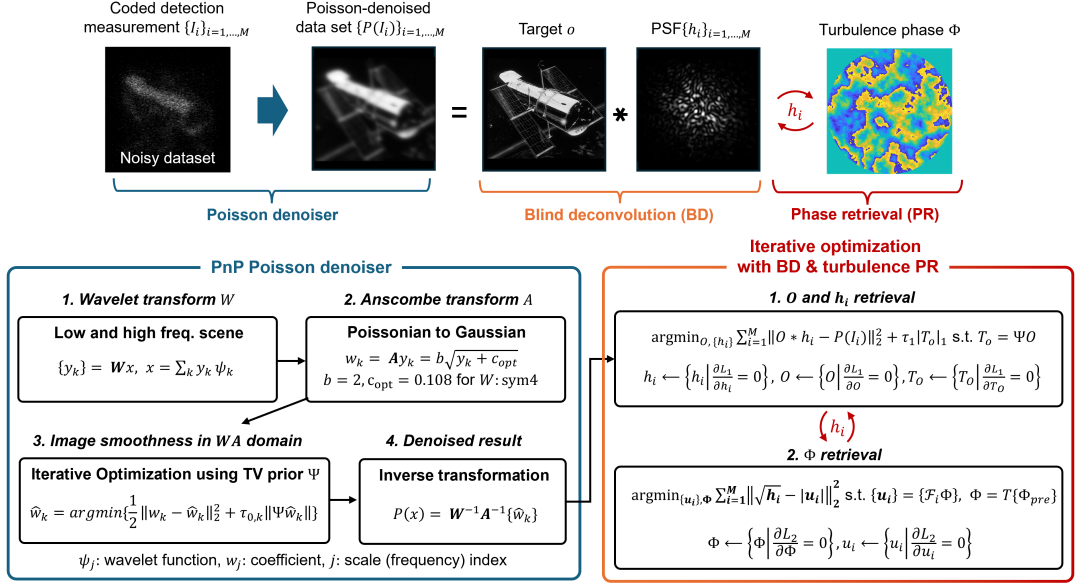

FIG. S2. Overview of the Turbulence-Aware Poisson Blind Deconvolution (TAP-BD) framework. The process begins with PnP Poisson denoising, transforming noisy measurements into a denoised dataset. This is followed by blind deconvolution (BD), which reconstructs the target  $O$  and the set of PSFs  $\{h_i\}$ . Turbulence phase retrieval (PR) then refines the turbulence phase  $\Phi$  using the intermediate PSFs  $\{h_i\}$  estimated in the BD stage. BD and PR are iteratively optimized, leveraging the denoised inputs to achieve robust reconstruction under low-photon conditions.

### A. Poisson denoiser

To stabilize reconstruction under severe shot noise, TAP-BD applies a Poisson denoiser in the PnP step, transforming noisy inputs  $\{I_i\}$  into denoised data  $\{P_i\}$ , following [1]. This step reduces noise across photon levels and complements Gaussian-optimized TV regularization without requiring extensive tuning.

The denoiser first applies wavelet decomposition  $\mathbf{W}$  to the raw Poissonian measurement  $x$ , separating it into frequency bands:

$$\{y_k\}_{k=1,\dots,K} = \mathbf{W}x, \quad x = \sum_k y_k \psi_k, \quad (\text{S4})$$

where  $\psi_k$  is the wavelet function (here, sym4),  $\{y_k\}$  are the 2D wavelet coefficients, and  $k$  indexes frequency bands. Only the first (LL) and last (HH) frequency components are used.

Next, the wavelet-based data undergoes the Anscombe transform  $\mathbf{A}$  to map the Poissonian measurements to the Gaussian domain for improved noise handling:

$$w_k = \mathbf{A}y_k = b\sqrt{y_k + c_{\text{opt}}}, \quad (\text{S5})$$

Where  $b = 2$  and  $c_{\text{opt}} = 0.108$  are fixed parameters for sym4, following [1].

The transformed wavelet coefficient  $\{w_k\}$  are then smoothed using TV regularization to remove noise effect while preserving essential details:

$$\hat{w}_k = \argmin \frac{1}{2} \|w_k - \hat{w}_k\|_2^2 + \tau_{0,k} \|\Psi \hat{w}_k\|, \quad (\text{S6})$$

where  $\Psi$  is the TV operator and  $\tau_{0,k}$  controls smoothness based on mean photons level.

Finally, the inverse Anscombe and wavelet transforms restore the denoised data:

$$P(x) = \mathbf{W}^{-1} \mathbf{A}^{-1} \{\hat{w}_k\}, \quad (\text{S7})$$

This step stabilizes reconstruction across photon levels by reducing sensitivity to hyperparameter settings (Fig. S3). At high photon counts, however, the denoiser may slightly degrade image quality [1].

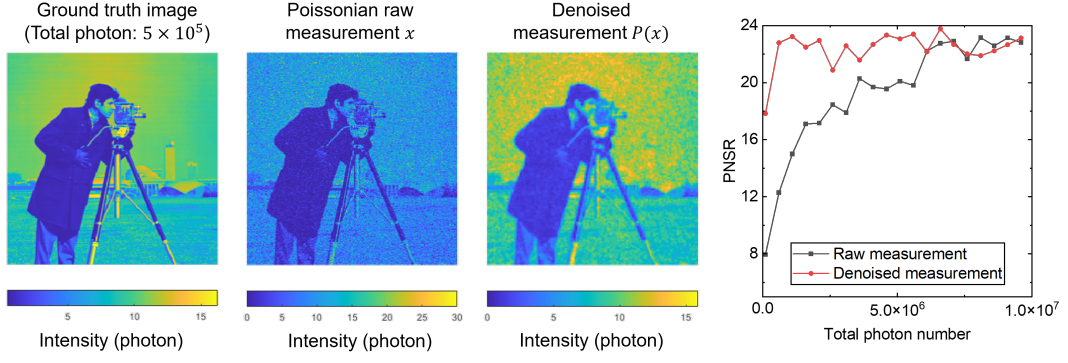

FIG. S3. Poisson denoiser effectively reduces shot noise in the low-photon regime, significantly improving PSNR and preserving key image features.

### B. Blind deconvolution (BD)

In the BD framework, the optimization problem seeks to jointly estimate the target  $O$  and a set of PSFs  $\{h_i\}$  from the denoised measurements  $\{P_i\}$ . The reconstruction of the single target  $O$  acts as a consistency constraint across measurements  $\{P_i\}$ , improving PSFs estimation by ensuring they align with the same target  $O$ . In the BD framework, the objective function is:

$$\operatorname{argmin}_{O, \{h_i\}_{i=1, \dots, M}} \sum_{i=1}^M \left[ \frac{1}{2} \|h_i * O - P_i\|^2 \right] + \tau_1 \|T_O\|, \quad \text{s.t. } T_O = \Psi O, \quad (\text{S8})$$

where  $P_i = P(I_i)$  represents the denoised measurements from the Poisson denoiser on the observed data  $I_i$ . Here,  $T_O$  is an auxiliary variable subject to TV regularization, and  $\Psi$  is the TV operator. The operator  $\Psi O$  produces two images representing vertical and horizontal differences, expressed as:

$$\Psi O_{i,j} = \begin{bmatrix} O_{i+1,j} - O_{i,j} \\ O_{i,j+1} - O_{i,j} \end{bmatrix}. \quad (\text{S9})$$

Using the augmented Lagrangian approach, we transform this constrained optimization problem into an unconstrained form:

$$L_1(O, T_O, \{h_i\}_{i=1, \dots, M}, \lambda_1) = \sum_{i=1}^M \left[ \frac{1}{2} \|h_i * O - P_i\|^2 \right] + \tau_1 \|T_O\| + \frac{\gamma_1}{2} \|T_O - \Psi O + \lambda_1\|^2, \quad (\text{S10})$$

where  $\lambda_1$  is a dual variable (Lagrange multiplier), and  $\gamma_1$  is the penalty parameter.

To solve for  $O$ ,  $T_O$ ,  $\{h_i\}$ , and  $\lambda_1$ , we apply the alternating direction method of multipliers (ADMM), which optimizes each variable sequentially while holding the others fixed. This iterative process updates each variable at the  $j$ -th iteration as follows:

$$O^{(j+1)} = \operatorname{argmin}_O L_1(O, T_O^{(j)}, \{h_i^{(j)}\}_{i=1, \dots, M}, \lambda_1^{(j)}) \quad (\text{S11})$$

$$T_O^{(j+1)} = \operatorname{argmin}_{T_O} L_1(O^{(j+1)}, T_O, \{h_i^{(j)}\}_{i=1, \dots, M}, \lambda_1^{(j)}) \quad (\text{S12})$$

$$\{h_i^{(j+1)}\}_{i=1, \dots, M} = \operatorname{argmin}_{\{h_i\}_{i=1, \dots, M}} L_1(O^{(j+1)}, T_O^{(j+1)}, \{h_i\}, \lambda_1^{(j)}) \quad (\text{S13})$$

$$\lambda_1^{(j+1)} = \lambda_1^{(j)} + \gamma_1 (T_O^{(j+1)} - \Psi O^{(j+1)}). \quad (\text{S14})$$

Here,  $\lambda_1$  is updated through a gradient ascent step, gradually enforcing constraint satisfaction in the augmented Lagrangian. While methods like stochastic gradient descent could be used, we employ closed-form solutions using stationary points to accelerate convergence. For analytical gradient calculation, we have to express each operation as

pointwise (or matrix multiplication in a diagonal form) in a specific basis. In the Fourier domain, the convolution term  $h_i * O$  simplifies to pointwise multiplication, expressed as:

$$\mathcal{F}\{h_i * O\} = \mathcal{F}\{h_i\} \cdot \mathcal{F}\{O\} \implies h_i * O = \mathcal{F}^{-1}\{\mathcal{F}\{h_i\} \cdot \mathcal{F}\{O\}\}. \quad (\text{S15})$$

To simplify gradients  $\frac{\partial L_1}{\partial O}$  and  $\frac{\partial L_1}{\partial h}$ , we shift to the Fourier domain, where convolutions become multiplications. Defining Fourier-transformed variables, e.g.,  $\tilde{x} = \mathcal{F}(x)$ , we rewrite  $L_1$  as:

$$L_1(\tilde{O}, \tilde{T}_O, \{\tilde{h}_i\}_{i=1,\dots,M}, \tilde{\lambda}_1) = \sum_{i=1}^M \left[ \frac{1}{2} \|\tilde{h}_i \tilde{O} - \tilde{P}_i\|^2 \right] + \tau_1 \|\tilde{T}_O\| + \frac{\gamma_1}{2} \|\tilde{T}_O - \tilde{\Psi} \tilde{O} + \tilde{\lambda}_1\|^2. \quad (\text{S16})$$

Setting  $\frac{\partial L_1}{\partial O} = 0$ , we obtain:

$$\frac{\partial L_1}{\partial \tilde{O}} = \sum_{i=1}^M \left[ (\tilde{h}_i^j)^H (\tilde{h}_i^j \tilde{O} - \tilde{P}_i) \right] - \gamma_1 \tilde{\Psi}^H (\tilde{T}_O^j - \tilde{\Psi} \tilde{O} + \tilde{\lambda}_1^j) = 0, \quad (\text{S17})$$

where  $(\tilde{h}_i^j)^H$  and  $\tilde{\Psi}^H$  are the Hermitian adjoint operators in the Fourier domain.

Rearranging this expression, the update rule for  $\tilde{O}$  is:

$$\tilde{O}^{(j+1)} = \left( \sum_{i=1}^M (\tilde{h}_i^j)^H \tilde{h}_i^j + \gamma_1 \tilde{\Psi}^H \tilde{\Psi} \right)^{-1} \left( \sum_{i=1}^M (\tilde{h}_i^j)^H \tilde{P}_i - \gamma_1 \tilde{\Psi}^H (\tilde{T}_O^j + \tilde{\lambda}_1^j) \right). \quad (\text{S18})$$

Applying the inverse Fourier transform, we recover:

$$O^{(j+1)} = \text{Re}(\mathcal{F}^{-1}(\tilde{O}^{(j+1)})). \quad (\text{S19})$$

The operation  $\tilde{\Psi}^H x = \mathcal{F}[\Psi^H x]$  represents the Fourier transform of the adjoint TV operator  $\Psi^H$ , which sums horizontal and vertical pixel differences. Specifically,  $\Psi^H O_{i,j}$  is given by:

$$\Psi^H O_{i,j} = (O_{i-1,j}^y - O_{i,j}^y) + (O_{i,j-1}^x - O_{i,j}^x). \quad (\text{S20})$$

To efficiently compute  $\tilde{\Psi}^H \tilde{\Psi}$  in the Fourier domain, one can define a Laplacian-like filter centered on the main pixel with offsets for adjacent pixels as:

$$\Psi^H \Psi = \begin{cases} 4, & \text{at } (0,0), \\ -1, & \text{at } (1,0), (-1,0), (0,1), (0,-1), \\ 0, & \text{otherwise.} \end{cases} \quad (\text{S21})$$

Then,  $\tilde{\Psi}^H \tilde{\Psi} = |\mathcal{F}[\Psi^H \Psi]|$ . Further details on implementing  $\Psi$  in ADMM are available at [2, 3].

For  $T_O$ , we optimize directly in the spatial domain, as it does not involve convolution terms. Setting  $\frac{\partial L_1}{\partial T_O} = 0$ , we derive the following update rule:

$$\frac{\partial L_1}{\partial T_O} = \tau_1 \text{sign}(T_O) + \gamma_1 (T_O - \Psi O^{(j+1)} + \lambda_1^{(j)}) = 0. \quad (\text{S22})$$

This simplifies to:

$$T_O^{(j+1)} = \text{sign}(\Psi O - \lambda_1) \max \left( 0, |\Psi O - \lambda_1| - \frac{\tau_1}{\gamma_1} \right). \quad (\text{S23})$$

Next, finding stationary points for  $h_i$  using a closed-form optimization yields a Wiener deconvolution-like update rule with  $\gamma_2$  as a stabilization term, similar to the noise power spectral density (PSD) in Wiener deconvolution:

$$\tilde{h}_i^{(j+1)} = \left( \sum_{i=1}^M (\tilde{O}^{(j+1)})^H \tilde{O}^{(j+1)} + \gamma_2 \right)^{-1} \left( \sum_{i=1}^M (\tilde{O}^{(j+1)})^H \tilde{P}_i \right) \quad (\text{S24})$$

Similar to the  $O$  update, by applying the inverse Fourier transform, we recover:

$$h_i^{(j+1)} = \text{Re}(\mathcal{F}^{-1}(\tilde{h}_i^{(j+1)})). \quad (\text{S25})$$

Note that the denoising capability can be adjusted using  $\gamma_2$ , but even a small amount of residual noise can significantly impact the subsequent phase retrieval updates. To address this more effectively, we introduced a PnP soft thresholding on  $h_i$  to suppress residual noise, followed by the  $h_i$  update rule. This PnP thresholding is applied as:

$$\hat{h}_i^{(j+1)} = \text{sign}(h_i^{(j+1)}) \max\left(0, |h_i^{(j+1)}| - \tau_2\right). \quad (\text{S26})$$

Also, if necessary, one can use additional constraint on  $h_i$  to prevent the tendency of  $h_i$  to go too far outward by additionally applying aperture constraint. This step further stabilizes the PSF estimation, resulting in potential improvement of reconstruction performance in turbulence phase retrieval (PR).

### C. Phase retrieval (PR)

In this PR module, we incorporate two main inputs: (1) An intermediate set of estimates  $\{\hat{h}_i\}$  from the previous BD module, (2) corresponding set of phase diversity patterns  $\{\Gamma_i\}$ .

The objective function of the PR framework is to reconstruct the complex e-field  $\Phi$  by solving:

$$\underset{\{u_i\}_{i=1,\dots,M}, \Phi}{\text{argmin}} \sum_{i=1}^M \frac{1}{2} \left\| \sqrt{\hat{h}_i} - |u_i| \right\|^2, \quad \text{s.t. } u_i = \mathcal{F}_i \Phi, \quad (\text{S27})$$

where  $u_i$  is an auxiliary PSF e-field at the image plane, and  $\mathcal{F}_i$  incorporates wave propagation with the  $i$ -th phase diversity pattern  $\Gamma_i$ . Using the augmented Lagrangian method, the constrained optimization problem is reformulated as:

$$L_2(\{u_i\}_{i=1,\dots,M}, \Phi) = \sum_{i=1}^M \frac{1}{2} \left\| \sqrt{\hat{h}_i} - |u_i| \right\|^2 + \frac{\gamma_3}{2} \|u_i - \mathcal{F}_i \Phi + \lambda_3\|^2 \quad (\text{S28})$$

One might notice that the angle of  $u_i$  is solely given by the second term, so:

$$\angle u_i = \angle(\mathcal{F}_i \Phi - \lambda_3). \quad (\text{S29})$$

To solve for  $|u_i|$ , we derive the stationary point of  $L_2$  with respect to  $|u_i|$  as:

$$\frac{\partial L_2}{\partial |u_i|} = -\left(\sqrt{\hat{h}_i} - |u_i|\right) + \gamma_3(|u_i| - |\mathcal{F}_i \Phi - \lambda_3|) = 0. \quad (\text{S30})$$

Leading to the update:

$$|u_i^{(j+1)}| = (1 + \gamma_3)^{-1} \left( \sqrt{\hat{h}_i^{(j+1)}} + \gamma_3 |\mathcal{F}_i \Phi^{(j)} - \lambda_3^{(j)}| \right) \quad (\text{S31})$$

Thus, the entire  $u_i$  is updated as:

$$u_i^{(j+1)} = (1 + \gamma_3)^{-1} \left( \sqrt{\hat{h}_i^{(j+1)}} + \gamma_3 |\mathcal{F}_i \Phi^{(j)} - \lambda_3^{(j)}| \right) \exp\left(j \angle \left( \mathcal{F}_i \Phi^{(j)} - \lambda_3^{(j)} \right)\right) \quad (\text{S32})$$

For a complex variable  $\Phi$ , we solve:

$$\frac{\partial L_2}{\partial \Phi} = \sum_{i=1}^M -\gamma_3 \mathcal{F}_i^H (u_i - \mathcal{F}_i \Phi + \lambda_3) = 0 \quad (\text{S33})$$

resulting in the closed-form update:

$$\Phi^{(j+1)} = \left( \sum_{i=1}^M \gamma_3 \mathcal{F}_i^H \mathcal{F}_i \right)^{-1} \left( \sum_{i=1}^M \gamma_3 \mathcal{F}_i^H (u_i^{(j+1)} + \lambda_3^{(j)}) \right) \quad (\text{S34})$$

Here,  $\mathcal{F}_i^H$  is the backpropagation operator, and  $\mathcal{F}_i^H \mathcal{F}_i = 1$ . The dual variable is updated via gradient ascent as:

$$\lambda_3^{(j+1)} = \lambda_3^{(j)} + \gamma_3 \left( u_i^{(j+1)} - \mathcal{F}_i \Phi^{(j+1)} \right) \quad (\text{S35})$$

$$(\text{S36})$$

By refining  $\Phi$  based on multiple intermediate PSF estimates and feeding it back to the BD as:

$$h_i^{(j+1)} = |\mathcal{F}_i \Phi^{(j+1)}|^2 \quad (\text{S37})$$

This alternating BD-PR update framework enables robust parameter estimation by integrating two distinct image formation models: incoherent convolution for the target and PSF recovery, and coherent wave propagation for turbulence phase retrieval. The pseudocode below outlines the PBD algorithm's iterative steps.

---

**Algorithm 1** Pseudocode for PBD algorithm

---

|                                  |                                                                                                                                                                                                                                                                                                                                                                                                                                                                                                                                                                                                                                                                                                                                                                                                                                                                                                                                                                                                                                                                                                                                                                                                                                                                                                                                                                                                                                                                                                                                                                                                                                                                                                                                                                                                                                                                                                                                                                                                                                                                                                                                                                                                                                                                           |
|----------------------------------|---------------------------------------------------------------------------------------------------------------------------------------------------------------------------------------------------------------------------------------------------------------------------------------------------------------------------------------------------------------------------------------------------------------------------------------------------------------------------------------------------------------------------------------------------------------------------------------------------------------------------------------------------------------------------------------------------------------------------------------------------------------------------------------------------------------------------------------------------------------------------------------------------------------------------------------------------------------------------------------------------------------------------------------------------------------------------------------------------------------------------------------------------------------------------------------------------------------------------------------------------------------------------------------------------------------------------------------------------------------------------------------------------------------------------------------------------------------------------------------------------------------------------------------------------------------------------------------------------------------------------------------------------------------------------------------------------------------------------------------------------------------------------------------------------------------------------------------------------------------------------------------------------------------------------------------------------------------------------------------------------------------------------------------------------------------------------------------------------------------------------------------------------------------------------------------------------------------------------------------------------------------------------|
| <b>Input:</b>                    | Multiple noisy measurements $\{I_i\}_{i=1,\dots,M}$ , and corresponding phase diversity patterns $\{\Gamma_i\}_{i=1,\dots,M}$ , hyperparameters $\tau_0 = [1 + 1/\bar{\mu}, 4 + 1/\bar{\mu}][1]$ , $\gamma_1 = 1e^{-2}$ , $\tau_1 = 1e^{-5}$ , $\gamma_1, \gamma_2 = 5e^{-6}$ , $\tau_2 = 3e^{-2}$ , $\gamma_3 = 1e^{-3}$ , where $\bar{\mu}$ is mean photon per pixel.                                                                                                                                                                                                                                                                                                                                                                                                                                                                                                                                                                                                                                                                                                                                                                                                                                                                                                                                                                                                                                                                                                                                                                                                                                                                                                                                                                                                                                                                                                                                                                                                                                                                                                                                                                                                                                                                                                   |
| <b>Output:</b>                   | Reconstructed target $O$ , PSFs $\{h_i\}_{i=1,\dots,M}$ , turbulence phase $\Phi$                                                                                                                                                                                                                                                                                                                                                                                                                                                                                                                                                                                                                                                                                                                                                                                                                                                                                                                                                                                                                                                                                                                                                                                                                                                                                                                                                                                                                                                                                                                                                                                                                                                                                                                                                                                                                                                                                                                                                                                                                                                                                                                                                                                         |
| <b>1. Initialization</b>         | Set $O^{(0)}$ , $\{h_i^{(0)}\}$ , $\Phi^{(0)}$ , $\{\lambda_1^{(0)}\}$ , $\lambda_3^{(0)}$ , initialize parameters and max_iter.                                                                                                                                                                                                                                                                                                                                                                                                                                                                                                                                                                                                                                                                                                                                                                                                                                                                                                                                                                                                                                                                                                                                                                                                                                                                                                                                                                                                                                                                                                                                                                                                                                                                                                                                                                                                                                                                                                                                                                                                                                                                                                                                          |
| <b>2. PnP Poisson Denoising</b>  | <p>For each noisy measurement <math>I_i</math>:</p> <p>Apply wavelet decomposition: <math>\{y_{i,k}\} = \mathbf{W}(I_i)</math> <span style="float:right">Eq. S5</span></p> <p>Apply Anscombe transform: <math>w_{i,k} = \mathbf{A}(y_{i,k})</math> <span style="float:right">Eq. S4</span></p> <p>Solve: <math>\hat{w}_{i,k} = \arg \min_{\hat{w}_{i,k}} \frac{1}{2} \ w_{i,k} - \hat{w}_{i,k}\ ^2 + \tau_{0,k} \ \Psi w_{i,k}\ </math> <span style="float:right">Eq. S6</span></p> <p>Reconstruct denoised data: <math>P_i = \mathbf{W}^{-1} \mathbf{A}^{-1} \{\hat{w}_{i,k}\}</math> <span style="float:right">Eq. S7</span></p>                                                                                                                                                                                                                                                                                                                                                                                                                                                                                                                                                                                                                                                                                                                                                                                                                                                                                                                                                                                                                                                                                                                                                                                                                                                                                                                                                                                                                                                                                                                                                                                                                                        |
| <b>3. Iterative Optimization</b> | <p>For <math>j = 1, \dots, \text{max\_iter}</math>:</p> <p><b>a. Blind Deconvolution (BD)</b></p> <p>Update target <math>O</math>:</p> $O^{(j+1)} = \mathcal{F}^{-1} \left( \left( \sum_{i=1}^M (\tilde{h}_i^j)^H \tilde{h}_i^j + \gamma_1 \tilde{\Psi}^H \tilde{\Psi} \right)^{-1} \left( \sum_{i=1}^M (\tilde{h}_i^j)^H \tilde{P}_i - \gamma_1 \tilde{\Psi}^H (\tilde{T}_O^j + \tilde{\lambda}_1^j) \right) \right)$ <span style="float:right">Eq. S18, S19</span> <p>Update target smoothness <math>T_O</math>:</p> $T_O^{(j+1)} = \text{sign}(\Psi O - \lambda_1) \max \left( 0,  \Psi O - \lambda_1  - \frac{\tau_1}{\gamma_1} \right)$ <span style="float:right">Eq. S23</span> <p>Update <math>\lambda_1</math>:</p> $\lambda_1^{(j+1)} = \lambda_1^{(j)} + \gamma_1 \left( T_O^{(j+1)} - \Psi O^{(j+1)} \right)$ <span style="float:right">Eq. S14</span> <p>Update PSFs <math>\{h_i\}</math>:</p> $h_i^{(j+1)} = \mathcal{F}^{-1} \left( \left( \sum_{i=1}^M (\tilde{O}^{(j+1)})^H \tilde{O}^{(j+1)} + \gamma_2 \right)^{-1} \left( \sum_{i=1}^M (\tilde{O}^{(j+1)})^H \tilde{P}_i \right) \right)$ <span style="float:right">Eq. S24, S25</span> <p>Apply PnP soft-thresholding on PSFs <math>\{h_i\}</math>:</p> $\hat{h}_i^{(j+1)} = \text{sign}(h_i^{(j+1)}) \max(0,  h_i^{(j+1)}  - \tau_2)$ <span style="float:right">Eq. S26</span> <p><b>b. Phase Retrieval (PR)</b></p> <p>Update auxiliary field <math>u_i</math>:</p> $u_i^{(j+1)} = (1 + \gamma_3)^{-1} \left( \sqrt{\hat{h}_i^{(j+1)}} + \gamma_3  \mathcal{F}_i \Phi^{(j)} - \lambda_3^{(j)}  \right) \exp \left( j \angle \left( \mathcal{F}_i \Phi^{(j)} - \lambda_3^{(j)} \right) \right)$ <span style="float:right">Eq. S32</span> <p>Update turbulence phase <math>\Phi</math>:</p> $\Phi^{(j+1)} = (M\gamma_3)^{-1} \left( \sum_{i=1}^M \gamma_3 \mathcal{F}_i^H (u_i^{(j+1)} + \lambda_3^{(j)}) \right)$ <span style="float:right">Eq. S34</span> <p>Update <math>\lambda_3</math> and <math>\lambda_4</math>:</p> $\lambda_3^{(j+1)} = \lambda_3^{(j)} + \gamma_3 \left( u_i^{(j+1)} - \mathcal{F}_i \Phi^{(j+1)} \right)$ <span style="float:right">Eq. S35</span> <p>Update PSFs: <math>h_i^{(j+1)} =  \mathcal{F}_i \Phi^{(j+1)} ^2</math> <span style="float:right">Eq. S37</span></p> |
| <b>4. Output</b>                 | Return $O$ , $\{h_i\}_{i=1,\dots,M}$ , and $\Phi$ .                                                                                                                                                                                                                                                                                                                                                                                                                                                                                                                                                                                                                                                                                                                                                                                                                                                                                                                                                                                                                                                                                                                                                                                                                                                                                                                                                                                                                                                                                                                                                                                                                                                                                                                                                                                                                                                                                                                                                                                                                                                                                                                                                                                                                       |

---

### III. OPTICAL CORRECTION FOR PHOTON-LIMITED IMAGING

Figure 4 in the main text shows that TAP-BD improves reconstruction, especially in low-photon regimes, when using the Poisson denoiser. While phase RMSE gains are modest and less intuitive, we validate their impact by applying the reconstructed phase for turbulence compensation and evaluating optical correction performance.

Figure S4 shows experimental results using a projected cameraman image and a  $20 \times$  lens. Without Poisson denoising (A), TAP-BD fails to recover meaningful details under  $< 1.07 \times 10^7$  photons. With denoising (B), essential phase features are preserved, enabling better optical correction despite only modest RMSE improvement (C, top). PSNR gains are significant—for instance, rising from 12 dB to 20 dB between  $0.32$  and  $2.10 \times 10^7$ . This suggests that the

denoiser helps the reconstructed phase retain critical features not fully captured by phase RMSE alone, underscoring its robustness in photon-starved conditions.

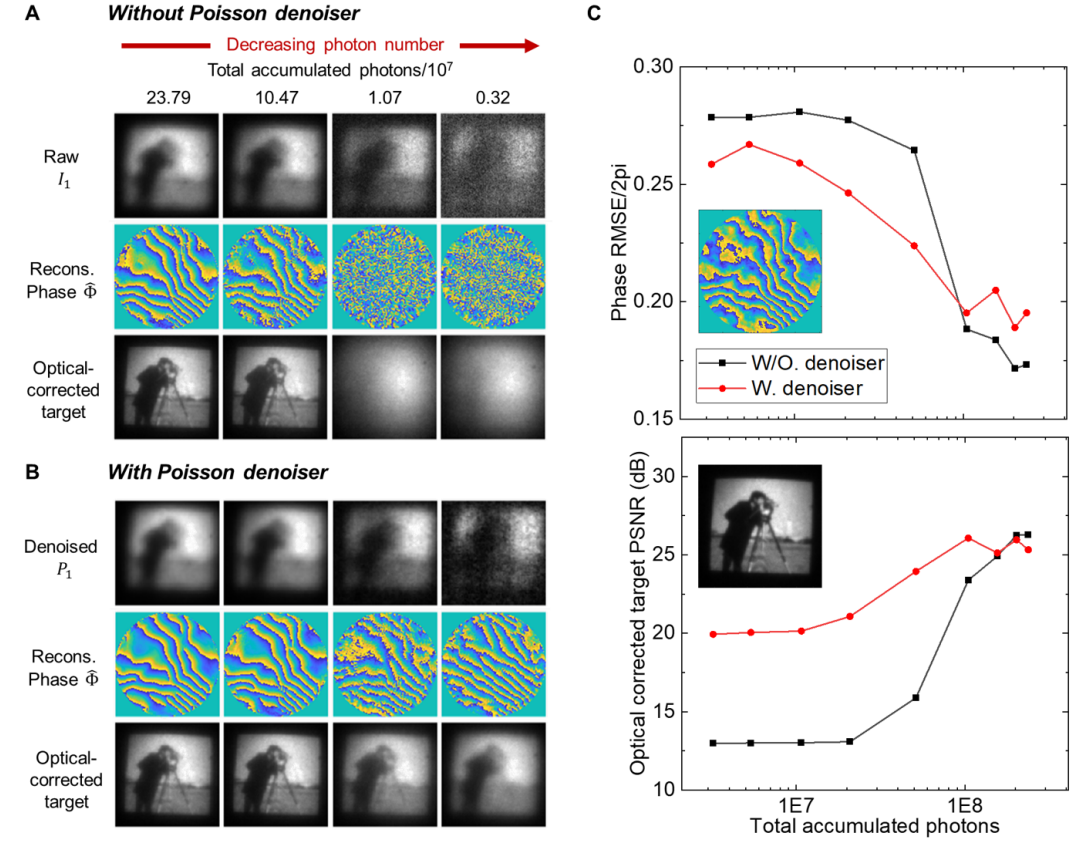

FIG. S4. Comparison of TAP-BD reconstruction with and without Poisson denoising under varying photon levels for a projected cameraman target. (A–B) From top to bottom: raw/denoised measurements, reconstructed phases, and optically corrected targets. The Poisson denoiser preserves key phase features in low-photon regimes, enabling improved correction. (C) Quantitative comparison of phase RMSE and corrected-target PSNR. Insets show ground truth phase and diffraction-limited target. All results use a 6 mm aperture, 48 SLM patterns, and 1000 iterations.

#### IV. LOSS LANDSCAPE

Figures 3 and 4 highlight key factors that boost reconstruction performance. Figure 3 shows that more measurements improve accuracy, while Figure 4 demonstrates the Poisson denoiser’s effectiveness in low-photon conditions. These trends align with intuition: additional measurements offer more information, and denoising mitigates shot noise (see also Figures S3, S4).

To better understand this, we analyzed the loss landscape by perturbing two components of the estimated turbulence phase  $\hat{\Phi}$ , generating PSFs  $\{h_i\}$  (Eq. S37), and evaluating the  $L_1$  loss terms (Eq. S10). Figure S5 shows that increasing measurements steepens and deepens the loss curvature, guiding optimization more effectively.

Figure S6 compares the loss landscape with and without the Poisson denoiser. Without the denoiser, particularly at low photon levels, the loss curvature becomes shallow, and multiple stationary points emerge, making convergence less reliable. In contrast, with the Poisson denoiser, the loss landscape exhibits well-defined minima, improving robustness, and ensuring more stable convergence.

[1] Y. Shen, Y. Chen, Q. Liu, S. Lou, W. Yu, X. Wang, and H. Chen, Improved anscombe transformation and total variation for denoising of lowlight infrared images, *Infrared Physics & Technology* **93**, 192 (2018).

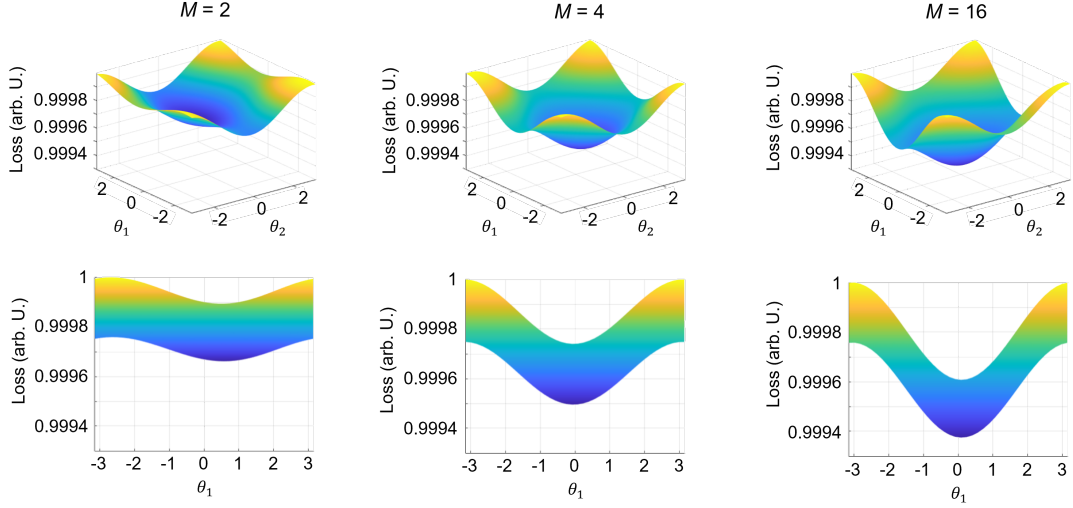

FIG. S5. Loss landscape vs. varying number of measurements. The landscape is derived by perturbing two phase parameters in reconstructed phase  $\hat{\Phi}$ , generating a corresponding set of PSFs  $\{h_i\}_{i=1,\dots,M}$ , which is then applied to the  $L_1$  (eq. S10). Increasing measurements gives deeper and steeper loss curvature, resulting in more precise guidance toward the minima.

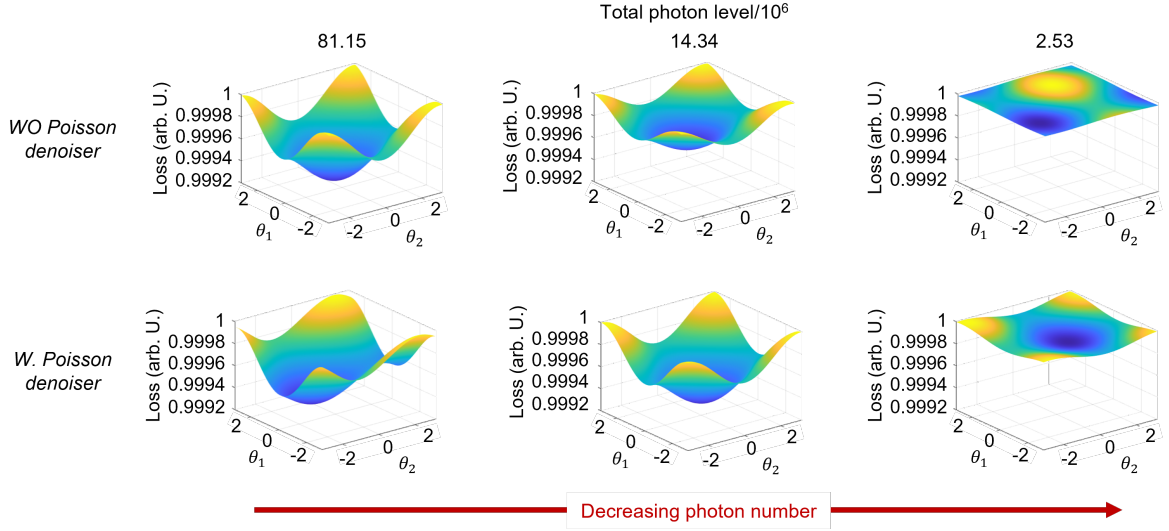

FIG. S6. Loss landscapes with and without the Poisson denoiser for varying photon numbers. The application of the Poisson denoiser stabilizes the loss landscape, providing deeper and well-defined minima, particularly in the low-photon regime ( $14.32 \times 10^6$  and  $2.53 \times 10^6$  total photons). However, in high-photon case ( $81.15 \times 10^6$  total photons), the Poisson denoiser does not necessarily improve the loss landscape, consistent with the observations in Fig. S3 and S4.

- [2] N. Antipa, G. Kuo, R. Heckel, B. Mildenhall, E. Bostan, R. Ng, and L. Waller, Diffusercam: lensless single-exposure 3d imaging, *Optica* **5**, 1 (2017).
- [3] N. Antipa, G. Kuo, R. Heckel, B. Mildenhall, E. Bostan, R. Ng, and L. Waller, Diffusercam, <http://www.laurawaller.com/research/diffusercam/> (2017), accessed: 2017-11-17.
